# Supplementary material for: A Successive-Elimination Approach to Adaptive Robotic Sensing
Source: arXiv:1809.10611 source file (2020-06-23)
Supplement: Supplementary file 1 [file appendix.tex]

%!TEX root = analysis_main.tex

\section{Parameter Estimation and Hypothesis Testing}
\label{subsec:parameter_estimation}

The source-seeking problem may be thought of as a large parameter estimation
problem, with unknown parameters $\{\mu(x)\}_{x \in \mc{S}}$. However, we need only
estimate the $\{\mu(x)\}$ to sufficient accuracy that we can reliably identify
the largest one. We formalize this idea of ``reliable identification'' within
the framework of hypothesis testing.

Identifying point $x^*$ as the source correctly with high probability is
equivalent to rejecting the null hypothesis that $\mu(x) < \mu(x^*), \forall x
\ne x^*$. To achieve an overall p-value of $\alpha_{\text{total}}$, we %must
apply a multiple test correction and lower the effective significance threshold
for each individual test. In particular, we use the Bonferroni-corrected
individual threshold given by $\alpha = \alpha_{\text{total}} / |\mc{S}|$.

In order to compute p-values for all $|\mc{S}|$ hypothesis tests, we must know the
distribution of our estimate for each of the $\{\mu(x)\}$. When presenting our
algorithm in the main body we simply assume the existence of
upper and lower confidence bounds for these estimators that correspond to
multiple test-corrected p-values. In the methods section, we present the
specific estimation scheme we use in order to compute these confidence
intervals. \comment{Fix these section references.}

\section{``Snake'' Pattern}
\label{subsec:snake_pattern}

Fig.~\ref{fig:snake_pattern} illustrates the ``snake'' pattern used in
$\snakeucb$ and $\naivesnake$ to sample radiation uniformly across the planar
environment. $\snakeucb$ could be applied in other environment configurations
and for other sensing tasks so long as there is an equivalent heuristic path
that samples the space approximately uniformly; finding such a path is generally
non-trivial.

\begin{figure}[ht]
  \centering
  \includegraphics[width=0.6\textwidth]{figures/snake_pattern.png}
  \caption{Illustration of the ``snake'' pattern used for approximate uniform
    sampling of the search space.}
  \label{fig:snake_pattern}
\end{figure}
