# Supplementary material for: A Successive-Elimination Approach to Adaptive Robotic Sensing
Source: arXiv:1809.10611 source file (2020-06-23)
Supplement: Supplementary file 2 [file arxiv_appendix.tex]

\documentclass{article}

% if you need to pass options to natbib, use, e.g.:
\PassOptionsToPackage{numbers, compress}{natbib}
% before loading nips_2018

% ready for submission
\usepackage{nips_2018}

% our things for definitions
\usepackage{amsthm}
\input{usepackage}
\input{notation}

% to compile a preprint version, e.g., for submission to arXiv, add
% add the [preprint] option:
% \usepackage[preprint]{nips_2018}

% to compile a camera-ready version, add the [final] option, e.g.:
% \usepackage[final]{nips_2018}

% to avoid loading the natbib package, add option nonatbib:
% \usepackage[nonatbib]{nips_2018}

\usepackage[utf8]{inputenc} % allow utf-8 input
\usepackage[T1]{fontenc}    % use 8-bit T1 fonts
\usepackage{hyperref}       % hyperlinks
\usepackage{url}            % simple URL typesetting
\usepackage{booktabs}       % professional-quality tables
\usepackage{amsfonts}       % blackboard math symbols
\usepackage{nicefrac}       % compact symbols for 1/2, etc.
\usepackage{microtype}      % microtypography
\usepackage{zref-xr, zref-user} % external references
\zexternaldocument*{main_nips}

\title{Appendix \\ {\small A Succcessive-Elimination Approach to Adaptive
    Sensing with Dynamic Agents}}

% The \author macro works with any number of authors. There are two
% commands used to separate the names and addresses of multiple
% authors: \And and \AND.
%
% Using \And between authors leaves it to LaTeX to determine where to
% break the lines. Using \AND forces a line break at that point. So,
% if LaTeX puts 3 of 4 authors names on the first line, and the last
% on the second line, try using \AND instead of \And before the third
% author name.

\author{
  David S.~Hippocampus\thanks{Use footnote for providing further
    information about author (webpage, alternative
    address)---\emph{not} for acknowledging funding agencies.} \\
  Department of Computer Science\\
  Cranberry-Lemon University\\
  Pittsburgh, PA 15213 \\
  \texttt{hippo@cs.cranberry-lemon.edu} \\
  %% examples of more authors
  %% \And
  %% Coauthor \\
  %% Affiliation \\
  %% Address \\
  %% \texttt{email} \\
  %% \AND
  %% Coauthor \\
  %% Affiliation \\
  %% Address \\
  %% \texttt{email} \\
  %% \And
  %% Coauthor \\
  %% Affiliation \\
  %% Address \\
  %% \texttt{email} \\
  %% \And
  %% Coauthor \\
  %% Affiliation \\
  %% Address \\
  %% \texttt{email} \\
}

\begin{document}
% \nipsfinalcopy is no longer used

\maketitle

\appendix

\input{analysis_intro}

\input{uniform_analysis}
\input{top_k_results}
\input{analysis_snake}
\input{analysis_naive}
%!TEX root = appendix_nips.tex
\section{Proof of Theorem~\ref{thm:snakeucb_runtime_topk} For Top-$k$ \label{sec:topkproof}}
In this section, we sketch the Proof of Theorem~\ref{thm:snakeucb_runtime_topk}. The proof is very similar to those of Theorem~\ref{thm:snakeucb} and Proposition~\ref{thm:snakeucb_runtime}, so we will focus on highlighting the major differences and added nuances. As in Proposition~\ref{thm:snakeucb_runtime}, the total run time is bounded by
\begin{eqnarray}
\tau_0\cardS \sum_{i \ge 0} \I(|\calS_i| + |\Stop_i| > k) +  \sum_{i \ge 0} 2^{i} |\calS_i| \I(|\calS_i| + |\Stop_i| > k)
\end{eqnarray}
Hence, our goal is to bound both the total number of rounds $\sum_{i \ge 0} \I(|\calS_i| + |\Stop_i| > k$, as well as the sample complexity $\sum_{i \ge 0} 2^{i} |\calS_i| \I(|\calS_i| + |\Stop_i| > k) $. We begin by observing that Lemma~\ref{lem:egood}, which states the event $\Egood$ defined as
\begin{eqnarray}
\forall i \ge 1, x \in \calS_i : \LCBbar_i(x) \le \LCB_i(x) \le \mu(x) \le \UCB_i(x) \le \UCBbar_i(x)~,
\end{eqnarray}
still holds with probability $1-\delta$ for the top-$k$ version of $\snakeucb$. 

	The following lemma is at the heart of our analysis:
	\begin{lemma}\label{lemtop_k_correct} $\Stop_i$ and $\calSi$ are disjoint for all rounds $i$. Moreover, suppose that for all rounds $i$ and all $x \in \calS_i$, the confidence intervals satisfy $\LCB_i(x) \le \mu(x) \le \UCB_i(x)$. Then $\Stop_i \subset \calS^*(k)$, and $\calS^*(k) \setminus \Stop_i \subset \calS_i$.
	\end{lemma}
	In other words, the update rules only add to $\Stop_i$ elements which are certain to be among the top-$k$, and only remove from $\calS_i$ elements which are certain to be ruled out from the top-$k$. Lemma~\ref{lemtop_k_correct} is proved in Sec.~\ref{proof_lemtop_k_correct}. In particular, on $\Egood$, we always have $\calS^*(k) \subset \calS_i \cup \Stop_i$, so that when the termination criterion $|\Stop_i| + |\calS_i| \le k$ occurs, $\Stop_i \cup \calS_i = \calS^*(k)$. This gives correctness under the event $\Egood$.

To analyze the stopping time, we first note that the quantities $\LCBbar_i(x)$ and $\UCBbar_i(x)$ are deterministic, and depend only on $\mu(x)$. Hence, we can define $\LCBbar_i^{(k)}$ and $\UCBbar_i^{(k+1)}$ to denote $\LCBbar_i(x^{+})$ and $\UCBbar_i(x^{(i)})$ for any $x^+,x^-$ with $\mu(x^+) \ge \mu^{(k)}$ and $\mu(x^-) \le \mu^{(k+1)}$.
\begin{lemma}\label{lemma:run_time_egood} Suppose that $\Egood$ holds, and $x \in \calS_i$. Then either $|\calS_i| + |\Stop_i| = k$ or $|\calS_i| + |\Stop_{i+1}| = k$, or otherwise $x \notin \calS_{i+1}$ as long as
\begin{eqnarray}
\begin{cases}
\LCBbar_i(x) > \UCBbar_i^{(k+1)} & \mu(x) \ge \mu(x^{(k)}) \\
\UCBbar_i(x) < \LCBbar_i^{(k)} & \mu(x) \le \mu(x^{(k+1)}) \\
\end{cases}
\end{eqnarray}
\end{lemma}
Since $\LCBbar$ and $\UCBbar$ are deterministic quantities, Lemma~\ref{lemma:run_time_egood} implies a deterministic upper bound on run-time under $\Egood$. Indeed, the total sample complexity is bounded by
\begin{eqnarray*}
&&\sum_{i \ge 0} 2^{i} |\calS_i| \I(|\calS_i| + |\Stop_i| > k) \le  \\
&&2\sum_{x \in \calS^*(k)} \inf\{2^i : \LCBbar_{i}(x) > \UCBbar^{(k+1)}_{i}(x)\}~ + 2\sum_{x \in \calS \setminus \calS^*(k)} \inf\{2^i : \UCBbar_{i}(x) < \LCBbar^{(k)}_{i}(x)\}~
\end{eqnarray*}
For $x \in \calS^*(k)$, we apply Proposition~\ref{prop:sample_comp} with $x_1 = x$ and $x_2$ such that $\mu(x_2) = \mu(x^{(k+1)})$. This gives that for any $x \in \calS^*(k)$,
\begin{eqnarray}\label{}
\inf\{2^i : \LCBbar_{i}(x) > \UCBbar^{(k+1)}_{i}(x)\} \lesssim C \left(\tau_0 + \frac{\mu(x) \log_+\left(\cardS \log_+\left(\frac{\mu(x)}{\Delta_{x;k}}\right)/\delta\right)}{\Delta_{x;k}^2}\right)
 \end{eqnarray}
and for any $x \in \calS \setminus \calS^*(k)$,
\begin{eqnarray}
 \inf\{2^i : \UCBbar_{i}(x) < \LCBbar^{(k)}_{i}(x)\} \lesssim C \left(\tau_0 + \frac{\mu^{(k)} \log_+\left(\cardS \log_+\left(\frac{\mu^{(k)}}{\Delta_{x;k}^2}\right)/\delta\right)}{\Delta_{x;k}^2}\right)
\end{eqnarray}
Summing the above two equations yields the first two terms in the bound given in Theorem~\ref{thm:snakeucb_runtime_topk}. For the last equation, we observe that by Lemma~\ref{lemma:run_time_egood}, the total number of rounds is given by
\begin{eqnarray*}
&&\max \left\{ \max_{x \in \calS \setminus \calS^*(k)}\inf \{i: \UCBbar_i(x) < \LCBbar_i^{(k)}\} , \max_{x \in \calS^*(k)}\inf \{i: \LCBbar_i(x) > \UCBbar_i^{(k+1)}\}  \right\} \\
&=& \max \left\{ \inf \{i: \UCBbar_i^{(k+1)} < \LCBbar_i^{(k)}\}, \inf \{i: \LCBbar_i^{(k)} > \UCBbar_i^{(k+1)}\}  \right\} \\
&=& \inf \{i: \UCBbar_i^{(k+1)} < \LCBbar_i^{(k)}\}\\
&\le&C \log \left(\tau_0 + \frac{\mu^{(k)} \log_+\left(\cardS \log_+\left(\frac{\mu^{(k)}}{(\mu^{(k)} - \mu^{(k+1)})^2}\right)/\delta\right)}{(\mu^{(k)} - \mu^{(k+1)})^2}\right)\\
&=& C \max_{x \notin \calS^*(k)}\log \left(\tau_0 + \frac{\mu^{(k)} \log_+\left(\cardS \log_+\left(\frac{\mu^{(k)}}{\Delta_{x;k}^2}\right)/\delta\right)}{\Delta_{x;k}^2}\right)~.
\end{eqnarray*}
Putting the pieces together concludes the proof.

\subsection{Proof of Lemma~\ref{lemma:run_time_egood}}
Let us first consider $x \in \calS_i$ with $\mu(x) \ge \mu^{(k)}$. Suppose $\Egood$ holds and $|\calS_i| > k - |\Stop_i|$ Then, there exists a point $x_- \in \calS_i \cap \{\calS \setminus \calS^*(k)\}$. Then $\mu(x_-) \le \mu^{(k+1)}$.  Since $\UCBbar_{i+1}(x)$ are monotone functions of $\mu(x)$, one has
\begin{eqnarray}
\UCB_{i}(x_-) \le \UCBbar_i(x_-) \le  \UCBbar_i^{(k+1)}
\end{eqnarray}
In particular, we find that
\begin{eqnarray}
	\mathrm{max}_{x' \in \calS_i}^{(k+1 - |\Stop_i|)} \UCB_{i}(x') \le \UCBbar_{i}^{(k+1)}
\end{eqnarray}
Hence, as soon as $\LCBbar_i(x) > \UCBbar_{i}^{(k+1)}$, 
\begin{eqnarray}
 \LCB_i(x) \ge \LCBbar_i(x) >  \UCBbar_{i}^{(k+1)} \ge \mathrm{max}_{x' \in \calS_i}^{(k+1 - |\Stop_i|)} \UCB_{i}(x')~,
	\end{eqnarray}
	so $x$ is removed from $\calS_i$ and placed in $\Stop_i$ by Equations~(\zref{eq:top_elim}) and~(\zref{eq:bot_elim}) in the main text.

Now consider $x \in \calS_i$ and $\mu(x) \le \mu^{(k+1)}$, and suppose that $|\calS_i| > k - |\Stop_{i+1}|$. Then there is an $x_+ \in \calS_i \cap \calS^*(k)$; $\mu(x_+) \ge \mu(x^{(k)}$, and thus $\LCB_i(x_+) \ge \LCBbar_i(x_+) \ge \LCBbar^{(k)}_i$. Thus, as soon as $\UCBbar_i(x) < \LCBbar_{i}^{(k)}$, then
\begin{eqnarray}
 \UCB_i(x) \le \LCBbar_i(x) <  \LCBbar_{i}^{(k+1)} \le \mathrm{max}_{x' \in \calS_i - \Stop_{i+1}}^{(k - |\Stop_{i+1}|)} \LCB_{i}(x')\}  ~,
	\end{eqnarray}
	so $x$ is removed from $\calS_i$ by Equation~(\zref{eq:bot_elim}) in the main text.

\subsection{Proof of Lemma~\ref{lemtop_k_correct}} \label{proof_lemtop_k_correct}
	Assume inductively that with high probability over all rounds $i$ and all sources $x$, all elements of $\Stop_i$ are confidently among the top $k$ sources $\calS^*(k)$, and all elements of $\calS^*(k) \setminus \Stop_i$ are elements of the candidate set $\calS_i$. We will also use the notation $\max^{(j)} \{\cdot\}$ to denote the $j$-th largest element of the set $\{\cdot\}$.

	We may assume that $|\calS_i \cup \Stop_i| > k$.

	Let's first examine the update rule for $\Stop_i$. Under the assumption that $\LCB_i(x) \le \mu(x) \le \UCB_i(x)$ holds for all $x \in \calS_i$, we have that if $x \in \Stop_{i+1} \setminus \Stop_i$,
	\begin{eqnarray}
	\mu(x) \ge \LCB_i(x) > \mathrm{max}_{x' \in \calS_i}^{(k+1 - |\Stop_i|)} \UCB_{i+1}(x') \ge \mathrm{max}_{x' \in \calS_i}^{(k+1 - |\Stop_i|)} \mu(x')~.
	\end{eqnarray}
	This implies that $\mu(x)$ is greater than at least $\mu(x')$ for at least $|\calS_i| - (k - |\Stop_i|)$ elements $x' \in \calS_i$. Since there are precisely $|\calS_i| - (k - |\Stop_i|)$ members of $\calS_i$ which are in $\calS \setminus \calS^*(k)$, and these have the lowest means, the above conditions imply that $x$ is indeed in $\calS^*(k)$.

	Now let's examine the update rule for $\calS_i$. For ease of notation, define $\calS_i' := \calS_i \setminus \Stop_{i+1}$. If the confidence intervals are uniformly correct, then we have that if $x \in \Stop_{i+1} \setminus \calS'_i$,
	\begin{eqnarray}
	\mu(x) \le \UCB_i(x) < \mathrm{max}_{x' \in \calS_i'}^{(k - |\Stop_{i+1}|)} \LCB_{i+1}(x') \le \mathrm{max}_{x' \in \calS_i'}^{(k - |\Stop_{i+1}|)} \mu(x')~.
	\end{eqnarray}
	Thus, $\mu(x)$ is not among the top $k - |\Stop_{i+1}|$ true means in $\calS'$; and the $k - |\Stop_{i+1}|$ members of $\calS_i'$ which have the top means are precisely the elements of $\calS_i \cap \calS^*(k)$.

\input{concentration_proofs}
\input{lower_bounds}
\pagebreak
\bibliographystyle{plainnat}
\bibliography{references}

%\section*{Extra things.}

%\section*{Snake Algorithm}
%\input{algorithm_snake}
%\end{document}

\end{document}
